# Supplementary material for: Cracking the Quantum Advantage threshold for Gaussian Boson Sampling
Source: arXiv:2106.01445 source file (2022-07-07)
Supplement: Supplementary file 1 [file Supplimentary.pdf]

# Contents

|                                                              |   |
|--------------------------------------------------------------|---|
| Initial state . . . . .                                      | 2 |
| Output state . . . . .                                       | 3 |
| Grand-canonical and canonical ensembles in GBS . . . . .     | 5 |
| Moments . . . . .                                            | 5 |
| Inverse moment problem in GBS . . . . .                      | 8 |
| Sherman-Morrison formula for multiple determinants . . . . . | 9 |

## INITIAL STATE

Gaussian boson sampling (GBS) experiment is mixing single-mode squeezed light states in a  $m$ -mode linear interferometer and measuring them with output detectors. In our work, we consider only threshold detection case - when output detectors resolve one or more coming photons without counting their exact number.

Here we present the formalism that describes our polynomial-time algorithm for simulation of a GBS set-ups without imperfections in detail.

As input states, we consider single-mode squeezed vacuum (SMSV) state in an input mode that can be represented as

$$|SMSV\rangle = S(\xi)|0\rangle \quad (1)$$

where  $\xi = re^{i\phi}$  and  $S(\xi) = e^{(-\xi\hat{a}^{\dagger 2} + \xi^*\hat{a}^2)/2}$ . In the photon number basis

$$|SMSV\rangle_i = \frac{1}{\sqrt{\cosh(r_i)}} \sum_{n=0}^{\infty} \left( \frac{-e^{-i\phi} \tanh(r_i)}{2} \right)^n \frac{\sqrt{2n!}}{n!} |2n\rangle \quad (2)$$

or

$$|SMSV\rangle_i = \frac{1}{\sqrt{Z}} \sum_{n=0}^{\infty} A_{ii}^n \frac{\sqrt{2n!}}{n!} |2n\rangle \quad (3)$$

In this way, partition functions of  $m$  inputs is  $Z = \prod_{i=1}^m Z_i$ , where

$$Z_i = \langle SMSV | SMSV \rangle_i = \sum_{n=0}^{\infty} (A_{ii}^* A_{ii})^n \frac{2n!}{(n!)^2} \quad (4)$$

It can be seen that  $|A_{ii}|^2 = \lambda_i$ ,  $\lambda_i < 1/4$ , because

$$\frac{1}{\sqrt{1-4\lambda}} = 1 + \sum_{n=1}^{\infty} \frac{(-1)^n}{2^{2n}} \frac{2n!}{(n!)^2} (-4\lambda)^n = \sum_{n=0}^{\infty} \lambda^n \frac{2n!}{(n!)^2} \quad (5)$$

Thus, we can represent  $Z$  as

$$Z = \prod_{i=1}^m \sum_{n=0}^{\infty} \lambda_i^n \frac{2n!}{(n!)^2} = \prod_{i=1}^m (1 - 4\lambda_i)^{-1/2} = \frac{1}{\sqrt{\det(1 - 4A^*A)}} \quad (6)$$

## OUTPUT STATE

SMVSs transfer through a linear optical network so that mapping on the creation operator in  $i$ -th output channel is

$$b_i^\dagger = \sum_j M_{ij} a_j^\dagger \quad (7)$$

where  $a_j^\dagger$  is the creation operator of  $j$ -th input state and matrix  $M$  is

$$M_{ij} = \sum_k U_{ki} U_{kj} A_{kk} \quad (8)$$

and  $U$  is a matrix of the interferometer, which consist of beam splitters and phase shifters operators

$$U = \prod_l u_{PS}^{(l)} u_{BS}^{(l)} \quad (9)$$

where

$$u_{PS}^{(l)} = \begin{pmatrix} 1 & 0 & \cdots & 0 & \cdots & 0 & 0 & \cdots & 0 \\ 0 & 1 & \cdots & 0 & \cdots & 0 & 0 & \cdots & 0 \\ \vdots & \vdots & \ddots & \vdots & \ddots & \vdots & \vdots & \ddots & \vdots \\ 0 & \cdots & e^{i\phi_l} & 0 & \cdots & 0 & e^{-i\psi_l} & \cdots & 0 \\ 0 & \cdots & 0 & 1 & \cdots & 0 & 0 & \cdots & 0 \\ \vdots & \ddots & \vdots & \vdots & \ddots & \vdots & \vdots & \ddots & \vdots \\ 0 & \cdots & 0 & 0 & \cdots & 1 & 0 & \cdots & 0 \\ 0 & \cdots & e^{i\psi_l} & 0 & \cdots & 0 & e^{-i\phi_l} & \cdots & 0 \\ \vdots & \vdots & \ddots & \vdots & \ddots & \vdots & \vdots & \ddots & \vdots \\ 0 & 0 & \cdots & 0 & \cdots & 0 & 0 & \cdots & 1 \end{pmatrix}$$

$$u_{BS}^{(l)} = \begin{pmatrix} 1 & 0 & \cdots & 0 & \cdots & 0 & 0 & \cdots & 0 \\ 0 & 1 & \cdots & 0 & \cdots & 0 & 0 & \cdots & 0 \\ \vdots & \vdots & \ddots & \vdots & \ddots & \vdots & \vdots & \ddots & \vdots \\ 0 & \cdots & \cos(\alpha_l) & 0 & \cdots & 0 & \sin(\alpha_l) & \cdots & 0 \\ 0 & \cdots & 0 & 1 & \cdots & 0 & 0 & \cdots & 0 \\ \vdots & \ddots & \vdots & \vdots & \ddots & \vdots & \vdots & \ddots & \vdots \\ 0 & \cdots & 0 & 0 & \cdots & 1 & 0 & \cdots & 0 \\ 0 & \cdots & -\sin(\alpha_l) & 0 & \cdots & 0 & \cos(\alpha_l) & \cdots & 0 \\ \vdots & \vdots & \ddots & \vdots & \ddots & \vdots & \vdots & \ddots & \vdots \\ 0 & 0 & \cdots & 0 & \cdots & 0 & 0 & \cdots & 1 \end{pmatrix}$$

In this way,  $M^\dagger M$  is a Hermit matrix, which can be diagonalized by  $V, V^T = V^\dagger$ . Take diagonal matrix  $E$ , which is given by  $E = V^T M V$ , so that

$$E^\dagger E = V^\dagger M^\dagger V^\dagger V^T M V = V^\dagger M^\dagger M V \quad (10)$$

$E^\dagger E$  is a diagonal eigenvalues matrix of  $M^\dagger M$ .

The partition function of a GBS output state is

$$Z = \prod_{i=1}^m \sum_{n=0}^{\infty} (E^* E)_i^n \frac{2n!}{(n!)^2} = \prod_{i=1}^m (1 - 4(E^* E)_i)^{-1/2} = \frac{1}{\sqrt{\det(1 - 4M^* M)}} \quad (11)$$

Thus, a state that corresponds to all outcomes with no photons in the  $i$ -th channel

$$|\Psi_i\rangle = |0_i\rangle \langle 0_i | \Psi \rangle = \frac{1}{\sqrt{Z}} e^{-M_{ij}^k b_i^\dagger b_j^\dagger} |0\rangle \quad (12)$$

$M^k$  equals  $M$  with vanished  $k$ -column and row

In this way, there is a polynomial way to calculate single-particle averages

$$d^k = \frac{Z_k}{Z} = \frac{\det(1 - 4M^{k*} M^k)^{-1/2}}{Z} \quad (13)$$

$$d^{ij} = \frac{Z_{ij}}{Z} = \frac{\det(1 - 4M^{ij*} M^{ij})^{-1/2}}{Z} \quad (14)$$

$M^{ij}$  equals  $M$  with vanished  $i$  and  $j$ -columns and rows

$$\bar{N} = \sum_k (1 - d^k) \quad (15)$$

$$\overline{\Delta N} = \overline{N^2} - \bar{N}^2 = \bar{N} + \sum_{i \neq j} (1 - d^i - d^j + d^{ij}) - \bar{N}^2 \quad (16)$$

## GRAND-CANONICAL AND CANONICAL ENSEMBLES IN GBS

Since the photon number operator commutes with observables  $[\hat{b}^\dagger \hat{b}, \hat{b}^\dagger \hat{b}^\dagger] = 0$  and  $[\hat{b}^\dagger \hat{b}, \hat{b} \hat{b}] = 0$ , Gaussian state of the entire system can be described by

$$|\Psi\rangle = \sum_n |2n\rangle \langle 2n|\Psi\rangle = \sum_n |2n\rangle \langle 2n| \frac{1}{\sqrt{Z}} e^{-M\hat{b}^\dagger{}^2} |0\rangle = \frac{1}{\sqrt{Z}} \sum_n \delta(2n - \hat{b}^\dagger \hat{b}) e^{-M\hat{b}^\dagger{}^2} |0\rangle \quad (17)$$

$$\delta(2n - \hat{b}^\dagger \hat{b}) = \frac{1}{const} \sum_\nu e^{i\nu(2n - \hat{b}^\dagger \hat{b})} \quad (18)$$

Thus, the partition function is given by

$$Z = \sum_n \langle \Psi | 2n \rangle \langle 2n | \Psi \rangle = \sum_{n,\nu} e^{i2n\nu} \langle 0 | e^{-M^* \hat{b}^2} e^{i\nu \hat{b}^\dagger \hat{b}} e^{-M \hat{b}^\dagger{}^2} | 0 \rangle = \sum_{n,\nu} e^{i2n\nu} Z_\nu \quad (19)$$

where  $Z_\nu$  is a discrete Fourier series, given by

$$Z_\nu = \frac{1}{\sqrt{\det(I - 4e^{i\nu} M^* M)}} \quad (20)$$

## MOMENTS

As it was discussed above, the first moment equals

$$\bar{N} = \sum_k \left( 1 - \frac{Z_k}{Z} \right) \quad (21)$$

where  $Z_k$  is

$$\begin{aligned} Z^k &= \det(1 - 4M^{k*} M^k)^{-1/2} \\ Z &= \det(1 - 4M^* M)^{-1/2} \end{aligned} \quad (22)$$

$M^k$  equals  $M$  with vanished  $i$ -column and  $i$ -row.

The second moment is

$$\begin{aligned} \overline{\Delta N} &= \overline{N^2} - \bar{N}^2 = \sum_{ij} n_i n_j - \bar{N}^2 = \\ &= \sum_i n_i^2 + 2 \sum_{i < j} n_i n_j - \bar{N}^2 \end{aligned} \quad (23)$$

If two detectors  $i, j$  clicked and we do not know what happens with others (they could click or not), the probability of this event is  $p_{11}$  ( $n_i n_j = p_{11}$ ). In the same way, if  $i, j$  detectors did not click, the probability equals  $p_{00}$ , and  $i$  detector clicked and  $j$  did not is  $p_{10}$ , vise versa -  $p_{01}$ .

$$p_{00} + p_{01} = \frac{Z_i}{Z}, p_{00} + p_{10} = \frac{Z_j}{Z}, p_{00} = \frac{Z_{ij}}{Z} \quad (24)$$

or

$$\begin{aligned} p_{01} &= \frac{Z_i}{Z} - \frac{Z_{ij}}{Z} \\ p_{10} &= \frac{Z_j}{Z} - \frac{Z_{ij}}{Z} \end{aligned} \quad (25)$$

Obviously,

$$p_{00} + p_{01} + p_{10} + p_{11} = 1 \quad (26)$$

Thus,

$$p_{11} = 1 - \frac{Z_i}{Z} - \frac{Z_j}{Z} + \frac{Z_{ij}}{Z} \quad (27)$$

The second moment equals

$$\overline{\Delta N} = \bar{N} + 2 \sum_{i \neq j} \left( 1 - \frac{Z_i}{Z} - \frac{Z_j}{Z} + \frac{Z_{ij}}{Z} \right) - \bar{N}^2 \quad (28)$$

At the same way, the third moment is given by

$$\begin{aligned} \mu &= \overline{N^3} + 3\bar{N}\overline{N^2} + \bar{N}^3 = \\ &= \sum_k n_k^3 + 6 \sum_{i < j} n_i^2 n_j + 6 \sum_{i \neq j \neq k} n_i n_j n_k + 3\bar{N}\overline{N^2} + \bar{N}^3 = \\ &= \sum_k n_k + 6 \sum_{i < j} n_i n_j + 6 \sum_{i \neq j \neq k} n_i n_j n_k + 3\bar{N}\overline{N^2} + \bar{N}^3 \end{aligned} \quad (29)$$

To find  $n_i n_j n_k = p_{111}$  we again write all possible probabilities for 3-detector clicking.

$$\begin{aligned} p_{000} + p_{001} + p_{010} + p_{011} &= \frac{Z_i}{Z} \\ p_{000} + p_{001} + p_{100} + p_{101} &= \frac{Z_j}{Z} \\ p_{000} + p_{010} + p_{100} + p_{110} &= \frac{Z_k}{Z} \\ p_{000} + p_{001} &= \frac{Z_{ij}}{Z} \\ p_{000} + p_{010} &= \frac{Z_{ik}}{Z} \\ p_{000} + p_{100} &= \frac{Z_{jk}}{Z} \\ p_{000} &= \frac{Z_{ijk}}{Z} \end{aligned} \quad (30)$$

or

$$\begin{aligned}
p_{100} &= \frac{Z_{jk}}{Z} - \frac{Z_{ijk}}{Z} \\
p_{010} &= \frac{Z_{ik}}{Z} - \frac{Z_{ijk}}{Z} \\
p_{001} &= \frac{Z_{ij}}{Z} - \frac{Z_{ijk}}{Z} \\
p_{110} &= \frac{Z_k}{Z} - \frac{Z_{ik}}{Z} - \frac{Z_{jk}}{Z} + \frac{Z_{ijk}}{Z} \\
p_{101} &= \frac{Z_j}{Z} - \frac{Z_{ij}}{Z} - \frac{Z_{jk}}{Z} + \frac{Z_{ijk}}{Z} \\
p_{011} &= \frac{Z_i}{Z} - \frac{Z_{ij}}{Z} - \frac{Z_{ik}}{Z} + \frac{Z_{ijk}}{Z}
\end{aligned} \tag{31}$$

$$p_{111} = 1 - \frac{1}{Z} \left( Z_i + Z_j + Z_k - Z_{ij} - Z_{jk} - Z_{ik} + Z_{ijk} \right) \tag{32}$$

and the third moment

$$\begin{aligned}
\mu &= \bar{N} + 6 \sum_{i \neq j} \left( 1 - \frac{Z_i}{Z} - \frac{Z_j}{Z} + \frac{Z_{ij}}{Z} \right) + \\
&+ 6 \sum_{i \neq j \neq k} \left( 1 - \frac{1}{Z} \left( Z_i + Z_j + Z_k - Z_{ij} - Z_{jk} - Z_{ik} + Z_{ijk} \right) \right) + 3\bar{N}\bar{N}^2 + \bar{N}^3
\end{aligned} \tag{33}$$

In this step, it is important to stress that the central moments and the cumulants are the same up to 4th moment. But for GBS problem is more appropriate to calculate the cumulants, because we want to estimate the quantity proportional to the size of a given system. We further will call them "moments" to refer to the inverse moment problem and avoid confusion.

The forth cumulant is

$$\eta = \bar{N}^4 - 4\bar{N}\bar{N}^3 - 3(\bar{N}^2)^2 + 12\bar{N}^2\bar{N}^2 - 6\bar{N}^4 \tag{34}$$

where

$$\begin{aligned}
\bar{N}^4 &= \sum_i n_i^4 + 8 \sum_{i < j} n_i^3 n_j + 6 \sum_{i < j} n_i^2 n_j^2 + 36 \sum_{i=k, j < l} n_i^2 n_j n_l + 24 \sum_{i \neq j \neq k \neq l} n_i n_j n_k n_l = \\
&= \sum_i n_i + 14 \sum_{i < j} n_i n_j + 36 \sum_{i \neq j \neq k} n_i n_j n_k + 24 \sum_{i \neq j \neq k \neq l} n_i n_j n_k n_l
\end{aligned} \tag{35}$$

as in calculating other moments,

$$\begin{aligned}
n_i n_j n_k n_l &= 1 - \frac{1}{Z} \left( Z_i + Z_j + Z_k + Z_l - Z_{ij} - Z_{jk} - Z_{kl} - Z_{ik} - Z_{il} - Z_{jl} + \right. \\
&\quad \left. + Z_{ijk} + Z_{jkl} + Z_{ikl} + Z_{ijl} - Z_{ijkl} \right)
\end{aligned} \tag{36}$$

## INVERSE MOMENT PROBLEM IN GBS

We have described way to calculate moments for an ideal GBS set-up. Here we show how this moments allow to estimate probability of any measurement outcome  $p(n)$ , where  $n$  - number of clicked detectors. According with the expressions (19),(20)  $p(n) = \sum_k p_k(n)$  probability of any measurement outcome is a sum over all sectors  $k$  at the  $n$  point, where  $p_k$  is a sector distribution, giving by

$$p_k(n) = \frac{1}{Z} \sum_q Z_q \quad (37)$$

where  $Z_q$  is partition function of a specific outcome,  $0 < q \leq 2^n$  - all possible detection outcomes. To calculate probabilities in this exact way require the exponential resources of a classical computer, which shows the initial complexity of GBS problem. But the sector distributions  $p_k$  have a clear unimodal form and can be approximated effectively by a limited number of moments because expressions of moments (21),(28),(33),(34) is also valid for sectors with replacement  $Z$  on  $Z_\nu$ .

Thus, we approximate each  $k$ -photon sector function using the formula

$$p_k(x) = c_k^0 e^{-(x-c_k^1)^2/2c_k^2} e^{c_k^3(x-c_k^1)^3/6(c_k^2)^3} e^{c_k^4(x-c_k^1)^4/8(c_k^2)^4} \quad (38)$$

Thus, we are able to iterative find the coefficients  $c_k^0, c_k^1, c_k^2, c_k^3, c_k^4$  via the calculated moments: on each step we change  $c_k^i$  slightly to obtain the right moment  $\overline{N}_k, \overline{\Delta N_k^2}, \mu_k, \eta_k$ . Here there exists the potential improvement of our method - it is possible to use another approximate expression for  $p_k$ , that would have less divergence on boundaries.

In summary, the most resource-intensive part of our algorithm is the calculations of moments: for the 4th order scheme, we need to compute all possible 4th-order minors of the initial matrix. In this work we also show that 4th-order algorithm runs using only  $n^5$  operations.

# SHERMAN-MORRISON FORMULA FOR MULTIPLE DETERMINANTS

Assume that we are given the matrix of the form  $R = \mathbb{I}_N + \sum_{jj'} |x_j\rangle a_{jj'} \langle y_{j'}|$  where  $\mathbb{I}$  is the  $N \times N$  identity matrix,  $x, y$  are some vector sets, and  $a$  is a square matrix of the size  $N' \times N'$ . Let us define the matrix  $b$  formed by scalar products of vectors  $x, y$  so that  $b_{j'j} = \langle y_{j'} | x_j \rangle$ . Then the determinant of  $R$  can be found as  $\det R = \det (\mathbb{I}_{N'} + ab)$ , where  $ab$  is the matrix product. For a small  $N'$  this allows for a very efficient calculation.

Let us apply this method to calculate the ratio of determinants appearing in the expression (6) of the article. Assume that we are given the matrix  $M$ . We consider a remove or, equally, vanishing, of the  $j$ th line and column in  $M$ . This corresponds to the transformation  $M \rightarrow M - M |j\rangle \langle j| - |j\rangle \langle j| M + |j\rangle \langle j| M |j\rangle \langle j|$ , where  $|j\rangle = (0, \dots, 0, 1, 0, \dots, 0)$  is a vector with the only non-zero element at the line  $j$ .  $M^\dagger$  is changed similarly. This way,  $A = 1 - 4e^{i\nu} M^\dagger M$  is changed to

$$A'_j = A + 4e^{i\nu} \begin{pmatrix} |j\rangle \\ M^\dagger |j\rangle \\ M^\dagger M |j\rangle \end{pmatrix} \begin{pmatrix} \langle j| M^\dagger M |j\rangle - \langle j| M^\dagger |j\rangle \langle j| M |j\rangle & \langle j| M^\dagger |j\rangle & -1 \\ \langle j| M |j\rangle & -1 & 0 \\ -1 & 0 & 0 \end{pmatrix} \begin{pmatrix} \langle j| \\ \langle j| M \\ \langle j| M M^\dagger \end{pmatrix}$$

Consequently,  $\det \frac{A'_j}{A} = \det R_j$  with

$$R_j = \mathbb{I}_3 + 4e^{i\nu} \begin{pmatrix} \langle j| M^\dagger M |j\rangle - \langle j| M^\dagger |j\rangle \langle j| M |j\rangle & \langle j| M^\dagger |j\rangle & -1 \\ \langle j| M |j\rangle & -1 & 0 \\ -1 & 0 & 0 \end{pmatrix} \times \\ \times \begin{pmatrix} \langle j| A^{-1} |j\rangle & \langle j| A^{-1} M^\dagger |j\rangle & \langle j| A^{-1} M^\dagger M |j\rangle \\ \langle j| A^{-1} M |j\rangle & \langle j| M A^{-1} M^\dagger |j\rangle & \langle j| M A^{-1} M^\dagger M |j\rangle \\ \langle j| A^{-1} M M^\dagger |j\rangle & \langle j| M M^\dagger A^{-1} M^\dagger |j\rangle & \langle j| M M^\dagger A^{-1} M^\dagger M |j\rangle \end{pmatrix}.$$

After nine matrices  $A^{-1}, \dots, M M^\dagger A^{-1} M^\dagger M$  are calculated, this allows to obtain  $\det \frac{A'_j}{A}$  for any  $j'$  as a determinant of a  $3 \times 3$  matrix. A removal of the two (three, four) lines-rows results in very similar expressions with the  $6 \times 6$  ( $9 \times 9$ ,  $12 \times 12$ ) matrices etc. Some extra optimization can be achieved by performing the calculations in the eigenbasis of  $M^\dagger M$ . The resulting number of operations required to calculate  $N^4$  four-rank moments at  $O(N)$  frequencies is about  $12^3 O(N^5)$ , where the prefactor reflects the complexity of the  $12 \times 12$  determinant calculation.
